# Supplementary material for: MaskSAM: Towards Auto-prompt SAM with Mask Classification for Volumetric Medical Image Segmentation
Source: arXiv:2403.14103 source file (2025-03-22)
Supplement: Supplementary file 1 [file X_suppl.tex]

\clearpage
\setcounter{page}{1}
\maketitlesupplementary

\section{Experiments with prompts from Ground Truth.}
To fairly compare and demonstrate the effectiveness of our model, we fine-tune it using accurate prompts generated from ground truth (GT) as input. In this version of the model, we remove the prompt generator and instead use the accurate prompts as input for the prompt encoder, while keeping the rest of the components unchanged from our MaskSAM model, including the designed adapters. 
Using accurate prompts from GT, our model achieves excellent performance, with a 94.70\% Dice and 94.30\% on Synapse and ACDC datasets, which outperform nnUNet by 8.5\% and 2.7\%, respectively. Furthermore, these results significantly surpass all existing SAM-based methods. These findings demonstrate that our designed adapters can effectively adapt SAM for medical image segmentation when provided with accurate prompts. Additionally, they show that, under the same conditions with accurate prompts, our model achieves near-perfect performance, significantly outperforming other SAM-based methods.

\section{Implementation Details}
Our models are based on the codebase of nnUNet for the preprocessing and postprocessing. For the preprocessing, we utilize some data augmentations such as rotation, scaling, Gaussian noise, Gaussian blur, brightness, and contrast adjustment, simulation of low resolution, gamma augmentation, and mirroring. During training, we set the initial learning rate to 0.01 and employ a ``poly'' decay strategy in Eq.~\eqref{equa:polydecay}.
\begin{equation}
    lr(e)= init\_lr \times (1 - \frac{e}{\rm MAX\_EPOCH})^{0.9},
\label{equa:polydecay}
\end{equation}
where $e$ means the number of epochs, MAX\_EPOCH means the maximum of epochs, set it to 500, 1000, and 1000 for ACDC, AMOS2022, and Synapse dataset respectively, and each epoch includes 250 iterations. 
We utilize SGD as our optimizer and set the momentum to 0.99. The weighted decay is set to 3e-5. For the postprocessing, we crop the whole image into several patches with half overlapping. For each patch, our model infers 8 times by different three axes~(\textit{i.e.} axial, sagittal, and coronal planes) and then averages all output to get the final predictions. All experiments are conducted using two NVIDIA RTX A6000 GPUs with 40GB memory with a batch size of 2.

\begin{table}[!b]\small
    \setlength{\tabcolsep}{3pt}
    \centering
    \vspace{-0.4cm}
    \resizebox{1\linewidth}{!}{ %< auto-adjusts font size to fill line
    \begin{tabular}{@{}l|cccccccccccc|c@{}}
    \toprule
    % Method & DSC & Aotra $\uparrow$ & Gallbladder $\uparrow$  & Kidnery(L) $\uparrow$ & Kidnery(R) $\uparrow$ & Liver $\uparrow$ & Pancreas $\uparrow$ & Spleen $\uparrow$ & Stomach  $\uparrow$ 
    % Method & Aot.$\uparrow$ & Gal.$\uparrow$  & Kid. L$\uparrow$ & Kid. R$\uparrow$ & Liv.$\uparrow$ & Pan.$\uparrow$ & Spl.$\uparrow$ & Sto.$\uparrow$  & DSC $\uparrow$\\
    Method & Spleen & R.Kd & L.Kd & GB & Eso. & Liver & Stomach & Aorta & IVC & Veins & Pancreas & AG & Average \\
    \midrule
    TransUNet & 95.2 & 92.7 & 92.9 & 66.2 & 75.7 & 96.9 & 88.9 & \textbf{92.0} & 83.3 & 79.1 & 77.5 & 63.7 & 83.8 \\ 
    nnUNet  & 94.2 & 89.4 & 91.0 & 70.4 & 72.3 & 94.8 & 82.4 & 87.7 & 78.2 & 72.0 & 68.0 & 61.6 & 80.2 \\
    3D UX-Net  & 94.6 & 94.2 & 94.3 & 59.3 & 72.2 & 96.4 & 73.4 & 87.2 & 84.9 & 72.2 & 80.9 & 67.1 & 81.4\\
    SwinUNETR  & 95.6 & 94.2 & 94.3 & 63.6 & 75.5 & 96.6 & 79.2 & 89.9 & 83.7 & 75.0 & 82.2 & 67.3  & 83.1\\
    nnFormer  & 93.5 & 94.9 & 95.0 & 64.1 & \textbf{79.5} & 96.8 & 90.1 & 89.7 & 85.9 & 77.8 & 85.6 & \textbf{73.9}  & 85.6\\
    SAMed\_h  & 95.3 & 92.1 & 92.9 & 62.1 & 75.3 & 96.4 & 90.2 & 87.6 & 79.8 & 74.2 & 77.9 & 61.0 & 82.1 \\
    % MA-SAM & 96.7 & 95.1 & 95.4 & 68.2 & \textbf{82.1} & 96.9 & \textbf{92.8} & \textbf{91.1} & 87.5 & \textbf{79.8} & 86.6 & 73.9 & 87.2 \\ 
    \hline
    MaskSAM (Ours)   & \textbf{97.0} & \textbf{95.3} & \textbf{95.3} & \textbf{68.6} & 78.3 & \textbf{97.3} & \textbf{92.4} & 91.8 & \textbf{87.6} & \textbf{80.4} & \textbf{86.9} & 72.3 & \textbf{86.9}
    \\
    \bottomrule
    \end{tabular}}
    \caption{Quantitative results on BTCV dataset. }% \caption
    \label{tab:btcv}
    \vspace{-0.4cm}
\end{table}

\section{Theoretical comparison with SAM-based models.} 
The main contributions of our MaskSAM different from the existing SAM-based models are i) \underline{automatic prompt}, ii) the classifier to generate \underline{semantic labels} for each mask, and iii) \underline{remain all parameters} of the original SAM for zero-shot capabilities. There are several categories of the existing SAM-based models. The first category does not modify SAM, such as MedSAM and Polyp-SAM. These models need manual prompts, such as points or boxes, and cannot classify masks into semantic labels. 
% Meanwhile, reference [r1] adopts U-Net to produce masks instead of manual prompts and just uses SAM without any modification. [r1] cannot classify masks into semantic labels and directly using SAM for medical image segmentation results in subpar performance.
% and exhibits imperfections or total failures in more challenging situations. 
The second category uses parameter-efficient transfer learning, such as Adapters, into SAM. The popular model, Med-SA, uses the GT to generate prompts during inference, which do not have any practical clinical values. It also includes the non-automatic models of the 3DSAM-Adapter and MA-SAM. These models do not handle the requirements of extra prompts. 
% Therefore, our model proposes a prompt generator module to solve this problem. 
The third category is that cannot classify masks into semantic labels, such as DeSAM, Med-SA, and MA-SAM. Since SAM only predicts binary masks, these models do not address the lack of classifiers. The fourth category is abandoning the components of SAM, such as Mask Decoder, to handle the inability to classify semantic labels, such as 3DSAM-Adapter. This way inevitably destroys the consistency and zero-shot capabilities of SAM. These models only use the pre-trained ViT encoder, which is not the contribution of SAM.

\section{More experiments.}
We conducted the experiments on the Beyond the Cranial Vault (BTCV) challenge
datase again but different split strategies and the Pancreas Tumor Segmentation task within 2018 MICCAI Medical Segmentation Decathlon Challenge (MSD-Pancreas) dataset.
We follow the split in SwinUNETR which contains 24 cases for training and 6 cases for testing for BTCV and the results are shown in Tab.~\ref{tab:pancreas}. We follow the split in 3DSAM-Adapter that the datasets are randomly split into 70\%, 10\%, and 20\% for
training, validation, and testing and the results are shown in Tab.~\ref{tab:btcv}. Our model achieves the state-of-the-art performance and outperforms nnUNet by 6.7\% and 1.0\% on BTCV and MSD-Pancreas dataset. Meanwhile, our model surpasses the SAM-based methods, SAMed\_h by 4.9\% on BTCV, MA-SAM by 2.4\% on MSD-Pancreas and 3DSAM-Adapter by 12.4\% on MSD-Pancreas dataset. In conclusion, the effectiveness of our method is robustly demonstrated.

\begin{table}[t]\small
    \makeatletter\def\@captype{table}\makeatother
    \centering
    \small
    \resizebox{0.5\linewidth}{!}{ %< auto-adjusts font size to fill line
    \begin{tabular}{@{}l|cc@{}}
    \toprule
    
     Methods & DSC $\uparrow$ & NSD $\uparrow$ \\
    \midrule
    
    nnUNet   & 41.6 & 62.5
    \\
    3D UX-Net  & 34.8 & 52.6
    \\
    SwinUNETR  & 40.6 & 60.0
    \\
    nnFormer   & 36.5 & 54.0 
    \\
    3DSAM-Adapter  & 30.2 & 45.4
    \\
    MA-SAM  & 40.2 & 59.1
    \\
    MaskSAM (Ours)  & \textbf{42.6} & \textbf{68.6}
    \\
    \bottomrule
    \end{tabular}}
    \caption{Quantitative results on MSD-Pancreas dataset.}% \caption
    \label{tab:pancreas}
    \vspace{-0.4cm}
\end{table}
